# Supplementary material for: Spatial Reasoning and Planning for Deep Embodied Agents
Source: arXiv:2409.19479 source file (2024-09-28)
Supplement: Supplementary file 1 [file calvin_iccv_appendix.pdf]

# Towards real-world navigation with deep differentiable planners

## Appendix A.

### A.1. Implicit assumptions of the VIN architecture

**Differences between VIN and the idealised VI on a grid.** Comparing eq. 1 in sec. 3 to eq. 2 in sec. 3.1, we note several differences:

1. The VIN value estimate  $V$  takes the maximum action-value  $Q$  across *all possible actions*  $\mathcal{A}$ , even illegal ones (e.g. moving into an obstacle). Similarly, the  $Q$  estimate is also updated even for illegal actions. In contrast, VI only considers legal actions for each state (cell), i.e.  $\mathcal{A}(i, j)$ .
2. The VIN reward  $\hat{R}$  is assumed independent of the action. This means that, for example, a transition between two states cannot be penalised directly; a penalty must be assigned to one of the states (regardless of the action taken to enter it).
3. The VIN transition probability is expanded into 2 terms,  $P^R$  which affects the reward and  $P^V$  which affects the estimated values. This decoupling means that they do not enjoy the physical interpretability of VI's  $P$  (i.e. probability of state transitions), and rewards and values can undergo very different transition dynamics.
4. Unlike the VI, the VIN considers the state transition translation-invariant. This means that it cannot model obstacles (illegal transitions) using  $\hat{P}$ , and must rely on assigning a high penalty to the reward  $\hat{R}$  of those states instead.

### A.2. Implementation details

#### A.2.1 Embodied pose states

One of our contributions is extending the VIN framework to accommodate embodied pose states, i.e. states which encode both position and orientation. We achieve this by augmenting the 2D state-space with an extra dimension for orientations. Table 1 shows correspondences between tensor dimensions of the positional method and the embodied method for each component of the architecture.  $X$  and  $Y$  are the size of the internal spatial discretisation of the environment,  $M$  is the internal discretisation of the orientation,  $A$  is the number of actions, and  $K$  is the kernel dimension for spatial locality.

Note that the value iteration step in CALVIN performs a 2D convolution of  $\hat{P}$  over a 2D value map in the case of positional states and a 3D convolution over a 3D value map with orientation in the case of embodied pose states. In the embodied case, the second dimension of  $\hat{P}$  corresponds to

the orientation of the current state, and the third dimension corresponds to that of the next state.

Table 1: Comparison of individual components in the implementation of CALVIN for positional states and for embodied pose states.

|                 | Positional            | Embodied                                |
|-----------------|-----------------------|-----------------------------------------|
| State $s$       | $(x, y)$              | $(\theta, x, y)$                        |
| VI step         | Conv2d                | Conv3d                                  |
| $V(s)$          | $X \times Y$          | $M \times X \times Y$                   |
| $Q(s, a)$       | $A \times X \times Y$ | $A \times M \times X \times Y$          |
| $\hat{A}(s, a)$ | $A \times X \times Y$ | $A \times M \times X \times Y$          |
| $\hat{P}$       | $A \times K \times K$ | $A \times M \times M \times K \times K$ |
| $\hat{R}$       | $A \times K \times K$ | $A \times M \times M \times K \times K$ |

#### A.2.2 Architectural design of Lattice PointNet

The Lattice PointNet described in sec. 4.2.2 consists of three stages: a CNN that extracts embeddings from observations in image-space (image encoder), a spatial aggregation step (eq. 10 in sec. 4.2.2) that performs max pooling of embeddings for each map cell, and another CNN that refines the map embedding (map encoder). The image encoder consists of two CNN blocks, each consisting of the following layers in order: batch normalisation, 2D convolution, dropout, ReLU and 2D max pooling. The map encoder consists of 2D convolution, dropout, ReLU, batch normalisation, and finally, another 2D convolution. The number of channels of each convolutional layer are (40, 20, 20, 20), respectively. The point clouds can consume a significant amount of memory for long trajectories. Hence, we sub-sampled the point embeddings to 50000 points after the image encoding step.

The input to the LPN is a 3-channel RGB image for the MiniWorld experiment, and a 128-channel embedding extracted using the first 2 blocks of ResNet18 pre-trained on ImageNet for the AVD experiment. For example-based navigation, an additional input of an example target image is given. We extract the ResNet18 embeddings for the target image, pass both the agent observation embeddings and the target embeddings through a  $1 \times 1$  convolutional layer and then take the dot product between the observation embed-

dings and the target embeddings. The dot product channel is then passed through another  $1 \times 1$  CNN and added to the output of the image encoder. This allows the network to learn the association between the target embedding and the observation embedding.

### A.2.3 Architectural design of the CNN backbone

This CNN backbone is used in a control experiment in appendix A.4.2 to show the effectiveness of the LPN backbone. In contrast to LPN which performs spatial aggregation of embeddings, the CNN backbone is a direct application of an encoder-decoder architecture that transforms image-space observations into map-space embeddings. Gupta *et al.* [1] employed a similar architecture to obtain their map embeddings. While they use ResNet50 as the encoder network, we used a simple CNN for the MiniWorld experiment to match the result obtained with LPN.

The CNN backbone consists of three stages: a CNN encoder, two fully-connected layers with ReLU to transform embeddings from image-space to map-space, and a CNN decoder. The encoder consists of 3 blocks of batch normalisation, 2D convolution, dropout, ReLU and 2D max pooling, and a final block with just batch normalisation and 2D convolution. The number of channels of each convolutional layer are (64, 128, 128, 128), respectively.

The fully-connected layers take in an input size of  $128 \times 5 \times 7$ , reduces it to a hidden size of 128, and outputs either  $128 \times 5 \times 5$  for the smaller maze or  $128 \times 4 \times 4$  for the larger maze, which is then passed to the decoder.

The decoder consists of 3 blocks of batch normalisation, 2D deconvolution, dropout and ReLU, and a final block with just 2D deconvolution. The number of channels of each deconvolution layers are (128, 128, 64, 20), respectively. The output size of the decoder depends on the map resolution, hence we chose appropriate strides, kernel sizes and paddings in the decoder network to match the output sizes of  $30 \times 30$  and  $80 \times 80$ . This approach is not scalable to maps with high resolution or with arbitrary size, which is one of the drawbacks of this approach.

## A.3. Experiment setup

### A.3.1 Expert trajectory generation

Expert trajectories are generated by running an A\* [2] planner from the start state to the target state. We assigned Euclidean costs to every transition in the 2D grid environments, and a cost of 1 per move for the MiniWorld and AVD environments. In the case of MiniWorld, an additional cost is assigned to locations near obstacles to ensure that the trajectories are not in close proximity to the walls.

### A.3.2 Hyperparameter choices

Similarly to VIN [4] which uses a 2-layer CNN to predict the reward map, and GPPN [3], which uses a 2-layer CNN to produce inputs to the LSTM, CALVIN uses a 2-layer CNN as an available actions predictor  $\hat{A}(s, a)$ . For each experiment, we chose the size of the hidden layer from  $\{40, 80, 150\}$ . For GPPN, 150 yielded the best results consistently. For VIN and CALVIN, 150 was used for all the grid environments, and 40 for MiniWorld and AVD, which yielded better navigation performance, presumably because the map embeddings are already learnt by the LPN.

VIN has an additional hyperparameter for the number of hidden action channels, which we set to 40, which is sufficiently bigger than the number of actual actions in all of our experiments. While the kernel size  $K$  for VIN and CALVIN were set to 3 for experiments in the grid environment, it was noted in [3] that GPPN works better with larger kernel size. Therefore, we chose the best kernel size out of  $\{3, 5, 7, 9, 11\}$  for GPPN. For experiments on MiniWorld and AVD, there are state transitions with step size of 2, hence we chose  $K = 5$  for VIN and CALVIN.

The number of value iteration steps  $k$  was chosen from  $\{20, 40, 60, 80, 100\}$ . For trajectory reweighting,  $\beta$  was chosen from  $\{0.1, 0.25, 0.5, 0.75, 1.0\}$ .

### A.3.3 Rollout at test time

We test the performance of the model by running navigation trials (rollouts) on a randomly generated environment. At every time step, the model is queried the set of  $Q$ -values  $\{Q(s, a) : a \in \mathcal{A}\}$  for the current state  $s$ , and an action which gives the maximum predicted  $Q$  value is taken.

While VIN is trained with  $V^{(0)}$  initialised with zeros, in a true Value Iteration algorithm, the value function must converge for an optimal policy to be obtained. To help the value function converge faster under a time and compute budget, we initialise the value function with predicted values from the previous time step at test time with online navigation.

We set a limit to the maximum number of steps taken by the agent, which were 200 for the fully-known  $15 \times 15$  grid, 500 for the partially known grid, 300 for MiniWorld ( $3 \times 3$ ), 1000 for MiniWorld ( $8 \times 8$ ), and 100 for AVD.

## A.4. Additional experiments

### A.4.1 Ablation study of removing loss components

CALVIN is trained on three additive loss components: a loss term for the predicted  $Q$ -values  $L_Q$  (sec.4.1.1), a loss term for the transition models  $L_P$  (sec.4.1.2), and a loss term for the action availability  $L_A$  (sec.4.1.3). We assessed the contribution of each loss component to the overall performance.

We conducted the experiments on the partially observable grid environment (sec.5.1.2). The results in table 2 indicate

that all loss components, in particular the transition model loss, contributes to the robust performance of the network.

Table 2: Navigation success rate of CALVIN in partially observable 2D mazes with loss components removed.

| Loss         | $L_Q + L_P + L_A$ | $L_Q + L_P$ | $L_Q + L_A$ |
|--------------|-------------------|-------------|-------------|
| Success rate | 0.88              | 0.82        | 0.08        |

#### A.4.2 Comparison of LPN against CNN backbone

We compared our proposed LPN backbone against a typical encoder-decoder CNN backbone as a component that maps observations to map embeddings. We evaluated the performance of the two methods for VIN, GPPN and CALVIN. In table 3, we observe that LPN backbone is highly effective, especially for larger environments where long-term planning based on spatially aggregated embeddings is necessary.

Table 3: Navigation success rate on unseen 3D mazes (Mini-World). Most methods do not generalise to larger mazes. The proposed LPN demonstrates robust performance in larger unseen mazes.

| Size         | CNN backbone |      |        | LPN backbone (ours) |      |             |
|--------------|--------------|------|--------|---------------------|------|-------------|
|              | VIN          | GPPN | CALVIN | VIN                 | GPPN | CALVIN      |
| $3 \times 3$ | 0.89         | 0.73 | 0.75   | 0.95                | 0.95 | <b>0.99</b> |
| $8 \times 8$ | 0.00         | 0.18 | 0.08   | 0.32                | 0.18 | <b>0.69</b> |

#### A.5. Learnt noisy transition model

CALVIN explicitly learns the transition model  $\hat{P}(s' - s|a)$  from expert trajectories. We confirm that this learning mechanism works even for transitions with added noise, which is the case for MiniWorld experiments. Figure 1 visualises the learnt state transitions for the *move forward* action. We observe that the network is able to model the noise added to transitions and propagate values probabilistically from the possible next states.

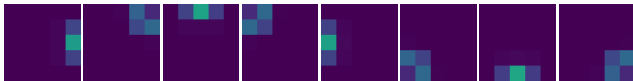

Figure 1: Transition model learnt from MiniWorld trajectories for the *move forward* action at each discretised orientation at  $45^\circ$  intervals. Higher values are brighter (yellow for a probability of 1), and lower values are darker (purple for a probability of 0).

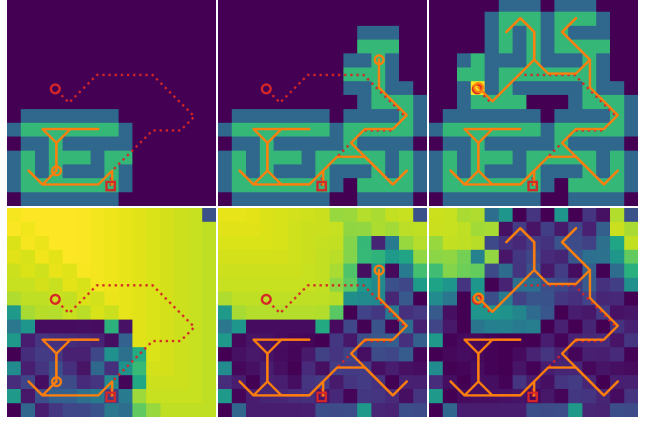

Figure 2: Example rollout of CALVIN after 21 steps (left column), 43 steps (middle column) and 65 steps (right column). CALVIN successfully terminated at 65 steps. **(top row)** Input visualisation: unexplored cells are dark, the discovered target is yellow. The correct trajectory is dashed, the current one is solid. The orange circle shows the position of the agent. **(bottom row)** Predicted values (higher values are brighter). Explored cells have low values, while unexplored cells and the discovered target are assigned high values.

#### A.6. Example rollout in a partially observable maze

We present an example of a trajectory taken by CALVIN at runtime, with corresponding observation maps and predicted values in Figure 2. At each rollout step, CALVIN performs inference on the best action to take based on its current observation map. No information about the location of the target is given until it is within view of the agent. This makes the problem challenging, since the agent may have to take significantly more steps compared to an optimal route to reach the target. In this example, the agent managed to backtrack every time it encountered a dead end, successfully reaching the target after 65 steps. The model initially assigns high values to all unexplored states. When the target comes into view, the model assigns a high probability to the availability of the “done” action at the corresponding state. The agent learns a sufficiently high reward for a successful termination so that the “done” action is triggered at the target.

#### A.7. Comparison of embodied navigation

For visual comparison of CALVIN, VIN and GPPN, we generated a maze and performed rollouts using each of the algorithms, assuming partial observability and embodied navigation.

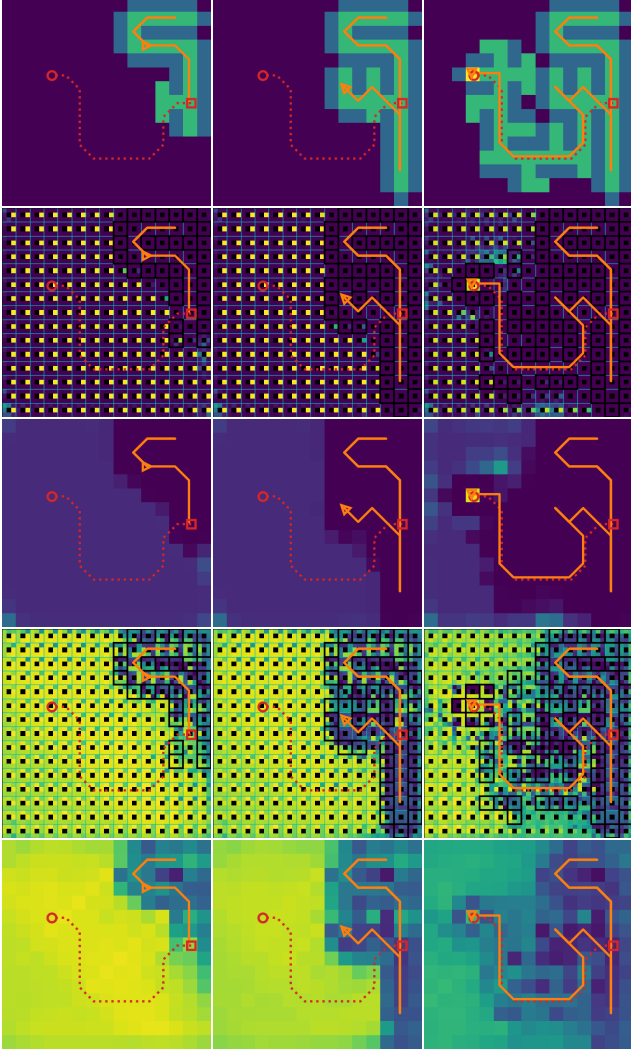

Figure 3: Example rollout of embodied CALVIN after 30 steps (left column), 60 steps (middle column) and 90 steps (right column). CALVIN successfully terminated at 91 steps. **(first row)** Input visualisation: unexplored cells are dark, the discovered target is yellow. The correct trajectory is dashed, the current one is solid. The orange triangle shows the position and the orientation of the agent. **(second row)** Predicted rewards (higher values are brighter). The 3D state-space (position/orientation) is shown, with rewards for the 8 orientations in a radial pattern within each cell (position). Explored cells have low rewards, while unexplored cells and the discovered target are assigned high rewards. **(third row)** Predicted rewards averaged over the 8 orientations. **(fourth row)** Predicted values following the same convention. Values are higher facing the direction of unexplored cells and the target (if discovered). **(fifth row)** Predicted values averaged over the 8 orientations.

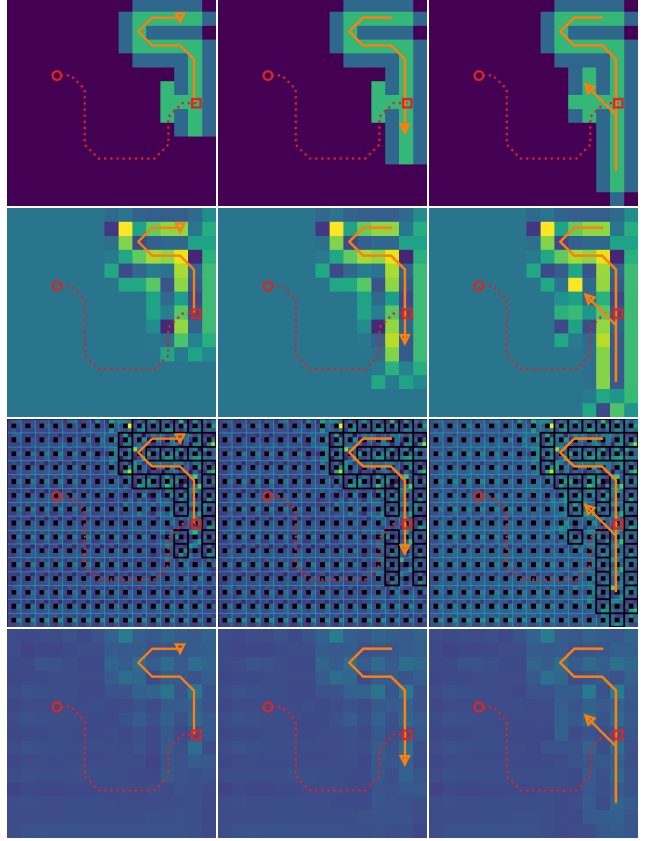

Figure 4: Example rollout of embodied VIN after 20 steps (left column), 40 steps (middle column) and 60 steps (right column). VIN kept oscillating between the same two states after 57 steps. The convention is the same as for fig. 2, except that a single reward map is shared across all orientations. **(first row)** Input visualisation. **(second row)** Predicted rewards. **(third row)** Predicted rewards averaged over the 8 orientations. **(fourth row)** Predicted values. **(fifth row)** Predicted values averaged over the 8 orientations.

#### A.7.1 Rollout of CALVIN

Figure 3 shows an example of a trajectory taken by CALVIN at runtime, with corresponding observation maps, predicted values and predicted rewards for taking the “done” action. Similarly to appendix A.6, the agent manages to explore unvisited cells and backtrack upon a dead end until the target is discovered. One key difference is that now the agent learns to predict rewards and values for every discretised orientation as well as the discretised location. Upon closer inspection, we observe that the predicted values are higher facing the direction of unexplored cells and towards the discovered target. Since rotation is a relatively low cost operation, in this training example, the network seems to have learnt to assign high rewards to a particular orientation at unexplored cells, from which high values propagate. Rewards and values averaged

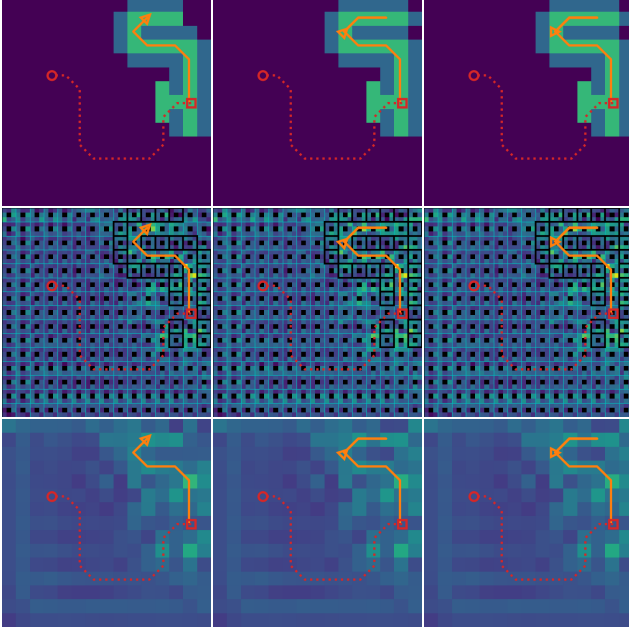

Figure 5: Example rollout of embodied GPPN after 15 steps (left column), 30 steps (middle column) and 45 steps (right column). GPPN revisits the same sequences of states leading to a dead end after 45 steps. The convention is the same as for fig. 2. **(first row)** Input visualisation. **(second row)** Predicted rewards. **(third row)** Predicted rewards averaged over the 8 orientations. **(fourth row)** Predicted values. **(fifth row)** Predicted values averaged over the 8 orientations.

over orientations yield a more intuitive visualisation.

### A.7.2 Rollout of VIN

A corresponding visualisation for VIN is shown in fig. 4. Unlike CALVIN’s implementation of rewards (eq. 5 in sec. 4.1) as a function of discretised states and actions, the “reward map” produced by the VIN does not offer a direct interpretation, as it is shared across all actions as implemented by Tamar *et al.* [4], and is also shared across all orientations in the case of embodied navigation. The values are also not well learnt, with some of the higher values appearing in obstacle cells. The unexplored cells are not assigned sufficiently high values to incentivise exploration by the agent. In this example, the agent gets stuck and starts oscillating between two orientations after 57 steps.

### A.7.3 Rollout of GPPN

Finally, a visualisation for GPPN is shown in fig. 5. Unlike VIN and CALVIN, GPPN does not have an explicit reward map predictor, but performs value propagation using an LSTM before outputting a final Q-value prediction.

Similarly to appendix A.7.2, the values predicted is not very interpretable, and does not incentivise exploration or avoidance of dead ends. In this example, the agent keeps revisiting a dead end that has already been explored in the first 20 steps.

## References

- [1] Saurabh Gupta, Varun Tolani, James Davidson, Sergey Levine, Rahul Sukthankar, and Jitendra Malik. Cognitive Mapping and Planning for Visual Navigation. In *Proceedings of the IEEE Conference on Computer Vision and Pattern Recognition*, 2017. arXiv: 1702.03920. 2
- [2] P. E. Hart, N. J. Nilsson, and B. Raphael. A formal basis for the heuristic determination of minimum cost paths. *IEEE Transactions on Systems Science and Cybernetics*, 1968. 2
- [3] Lisa Lee, Emilio Parisotto, Devendra Singh Chaplot, Eric Xing, and Ruslan Salakhutdinov. Gated Path Planning Networks. *arXiv:1806.06408 [cs, stat]*, June 2018. arXiv: 1806.06408. 2
- [4] Aviv Tamar, YI WU, Garrett Thomas, Sergey Levine, and Pieter Abbeel. Value Iteration Networks. In D. D. Lee, M. Sugiyama, U. V. Luxburg, I. Guyon, and R. Garnett, editors, *Advances in Neural Information Processing Systems 29*, pages 2154–2162, 2016. 2, 5
